# Supplementary material for: Weakly Supervised Bayesian Shape Modeling from Unsegmented Medical Images
Source: arXiv:2405.09697 source file (2024-05-15)
Supplement: Supplementary file 1 [file supplementary.tex]

\section*{Supplementary Material}

Supplementary material that may be helpful in the review process should
be prepared and provided as a separate electronic file. That file can
then be transformed into PDF format and submitted along with the
manuscript and graphic files to the appropriate editorial office.
